# Supplementary material for: Learning to Expand: Reinforced Pseudo-relevance Feedback Selection for Information-seeking Conversations
Source: arXiv:2011.12771 source file (2022-11-02)
Supplement: Supplementary file 1 [file appendix.tex]

\section{Appendix} \label{sec:appendix}
\subsection{Dataset Statistics and Pre-processing} \label{appendix:data_statistics}
The dataset statistics is shown in Table \ref{tab:exp_data_stat_train_valid_test}. For the MSDialog dataset, we removed some common prefixes such as “«AGENT»:” and use WordPiece~\citep{DBLP:journals/corr/WuSCLNMKCGMKSJL16} to tokenize the context and the response candidates for further modeling. For AliMe-CQA, the language of the context and response is Chinese and we use character-level tokenization for further modeling.

\subsection{PRF Term Candidates Retrieving} \label{appendix:candidates_retrive}
The goal of pseudo-relevance feedback (PRF) is to extract terms from the top-ranked documents during the retrieval process to help discriminate relevant documents from the irrelevant ones ~\cite{Cao:2008:SGE:1390334.1390377}. 

The expansion terms are extracted either according to the term distributions (e.g., extract the most frequent terms) or extracted from the most specific terms (e.g., extract terms with the maximum IDF weights) in feedback documents. Given the retrieved top $K_1$ QA posts $\mathcal{P}$ from the previous step, we compute a language model $\theta=P \left(w|\mathcal{P} \right)$ using $\mathcal{P}$. Then we extract the most frequent $K_2$ terms from $\theta$ as the PRF terms for the response candidate.
We first use the response candidate as the query to retrieve top $K_1$ QA posts from the external corpus with BM25 as the source of the external knowledge for each response candidate. While retrieving relevant documents, we perform several preprocessing steps including tokenization, punctuation removal, and stop word removal for the query. We set $K_1=10$ for MSDialog dataset, and $K_1=15$ for AliMe dataset. The external retrieval source corpus for MSDialog and AliMe are Stack Overflow data and unlabeled AliMe QA data respectively.
Once the response-relevant QA posts are retrieved for each response, we count the term frequencies for all terms in these posts and select the top $K_2$ frequent terms as the PRF terms for each response candidate. $K_2$ is set as $10$ for both the MSDialog dataset and the AliMe dataset.

Examples of retrieved PRF terms are shown in Table \ref{tab:prf_term_examples}. 
By analyzing these examples, we have the following observations: 
\begin{itemize}
    \item Those PRF terms that exactly shown in the responses are the \textit{key information} of the response, which is beneficial for ranking if those PRF terms are used to expand the response. For example, in the first case of  Table \ref{tab:prf_term_examples}, we find ``windows defender'' is the key information since the solution that response provided is to change the option of the ``windows defender''.
    \item Some PRF terms are not exactly shown in the response but have \textit{strong relevance} to the response which can fill the vocabulary gap between the context and the response if being used. For example, in the fourth case of Table \ref{tab:prf_term_examples}, even though the response does not mention the words ``antivirus'', ``security'', they are relevant to the response, which are helpful to be included in the context.
    \item Some PRF terms are \textit{less informative} or \textit{meaningless} for the response, which should be filtered. For example, in the second case of Table \ref{tab:prf_term_examples}, ``javascript'', ``chrome'' are irrelevant and may mislead the ranking model once expanded.
\end{itemize}

\subsection{Detailed Hyper-parameter Setting} \label{appendix:hyper_param}
We present the detailed hyper-parameters used for experiments.

 For the MSDialog dataset, the context length is truncated by 384 and the response length is truncated by 96. The batch size is set to 12. We use Adam optimizer with linear decay for both two models. The learning rate for BERT-Ranker is set to 3e-5 following the previous works.  For PRF-RL, we firstly pre-trained the BERT response ranker without PRF term selection of learning rate 3e-5 for 1000 steps, and then jointly trained the reinforced PRF term selector and the BERT response ranker with learning rate 1e-4, 1.5e-5 respectively. For reinforcement learning, we use max-pooling in the state representation, the number of the episode is set to 100, the reward discount reward factor is set to 0.3, and the reward set is randomly sampled from 0.5\% of the validation dataset considering the trade-off of quality and efficiency of training.

 For the AliMe dataset, the context length is truncated by 100 and the response length is truncated by 50. The batch size is set to 32. We again use Adam optimizer with linear decay for both two models. The learning rate for BERT-Ranker is set to 3e-5. For PRF-RL, we firstly pre-trained the BERT response ranker with a learning rate 3e-5 for 200 steps, and then jointly trained the reinforced PRF term selector and the BERT response ranker with a learning rate 1e-4, 5e-6 respectively. We again use max-pooling in the state representation, the number of the episode is set to 10, the reward discount reward factor is set to 0.3, and the reward set is randomly sampled from 1\% of the validation dataset.
 
\begin{table*}[h]
    \centering
    \caption{The examples of retrieved PRF Term candidates of MSDialog Dataset. Key information is colored \textit{{\color{red}red}}. Strong relevant terms are colored \textit{{\color{morange}orange}}. Other terms are less informative.}
    \begin{tabular}{p{12cm}|p{5cm}}
        \toprule
        \multicolumn{1}{c|}{Response} & \multicolumn{1}{c}{PRF-terms}\\ 
        \midrule
        Hello Hairy,  It appears that you're having issues with the Check apps and files option of your \keyterms{Windows defender}. For us to effectively assist you with your concern, we would like to know the following:   Regards. & \textit{{\color{red}windows}} \relevantterms{antivirus} powershell find installed \keyterms{defender} c urbancode udeploy groovy \\
        \midrule
        Hello,   Malware can be one of the factors why you're seeing this \keyterms{prompt}. For us to provide you the appropriate steps that can resolve your concern, we'd like to verify the following:   To have an eye view on the prompt that your seeing, we'd like to request for a screenshot of it.    Regards. & javascript using browser \keyterms{prompt} file expect \keyterms{security} \keyterms{administrator} user chrome \\
        \midrule
        It is unwise to suggest uninstalling an \keyterms{anti-virus} program. You have no information on the \keyterms{anti-virus} program currently residing on the computer. & \textit{{\color{red}antivirus}} error windows \keyterms{virus} file failed \relevantterms{backup} autoit outlook r \\
        \midrule
        Both are showing Avast still installed?  With Defender?   Some AV uninstall is known to be deficient, so then their users may have to hunt down the manufacturer's cleanup program.  I have no details for Avast. & \textit{{\color{morange}antivirus}} \relevantterms{security} \relevantterms{windows} blocked android java difference different apps \relevantterms{malware} \\
        \midrule
        It would seem this is the answer to all the questions about \keyterms{contacts} - Delete and create a new one.  Unfortunately I have added lots of personal details to each of my \keyterms{contacts}, which would be time consuming to re enter. There must be a better way, this 365 should save us time, not create more work - It is a simple operation in gmail! &
        create contact \relevantterms{email} \keyterms{contacts} users office sitecore \relevantterms{outlook} updating addresses \\
        \midrule
        Willems, do you have a \keyterms{crash} \keyterms{dump}? According to my Microsoft contacts, this issue has not yet been fixed, and they need a support case (can you open one?) or at the very least a \keyterms{crash} \keyterms{dump}. Thanks! & \textit{{\color{red}dump}} \keyterms{crash} windows c \relevantterms{debugging} \relevantterms{windbg} using outlook symbol capture \\
        \midrule
        The directions for adding the \keyterms{account} do not mention having to select MAPI or \keyterms{IMAP}. & \keyterms{imap} using \relevantterms{email} \relevantterms{outlook} \keyterms{account} folders python api specific vba \\
        \midrule
        Rufus has the code to \keyterms{boot} the machine. You have to have the \keyterms{USB} port as the first item in the \keyterms{BIOS} boot list. &
        \textit{{\color{red}usb}} \keyterms{boot} \relevantterms{bootable} drive windows \keyterms{bios} freenas \relevantterms{booting} hard nas \\
        \midrule
        Glenn\_k9, that is in-correct, when you \keyterms{run} the Command \keyterms{Prompt} it runs it as your normal user account access, for Administrator \keyterms{Privileges} you must right click and select Run as administrator see image below & \textit{{\color{morange}windows}} \relevantterms{admin} \keyterms{prompt} \keyterms{privileges} \keyterms{run} \relevantterms{running} without visual studio c \\
        \midrule
        How long have you been an \keyterms{Insider}? Did you read all of the information about Insiders when you signed up as an \keyterms{Insider}? Are you Slow ring or Fast ring? & windows asterisk uwp tiles \keyterms{insider} build download call unable band \\
        \bottomrule
    \end{tabular}
    \label{tab:prf_term_examples}
\end{table*}
